# Supplementary material for: In The Wild Ellipse Parameter Estimation for Circular Dining Plates and Bowls
Source: arXiv:2405.07121 source file (2024-05-12)
Supplement: Supplementary file 1 [file 12_appendix.tex]

\section{Appendix Section}
\label{sec:appendix_section}
Supplementary material goes here.
